# Supplementary material for: Enhancing Transformation-based Defenses using a Distribution Classifier
Source: arXiv:1906.00258 source file (2020-01-30)

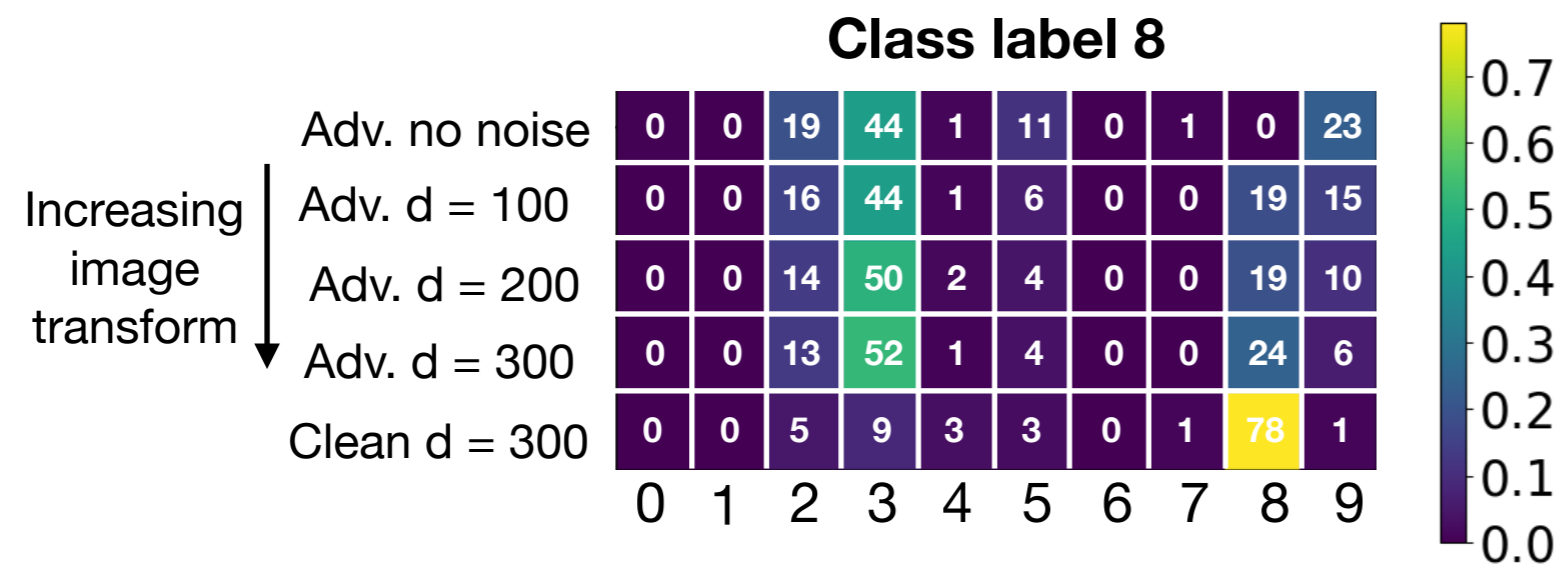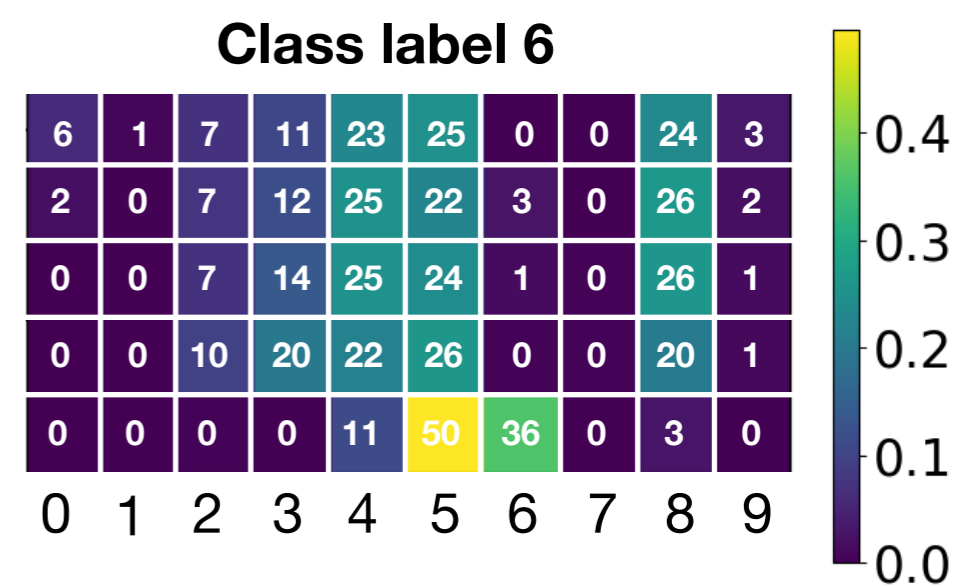

# MNIST, FGSM

## Increasing pixel deflections

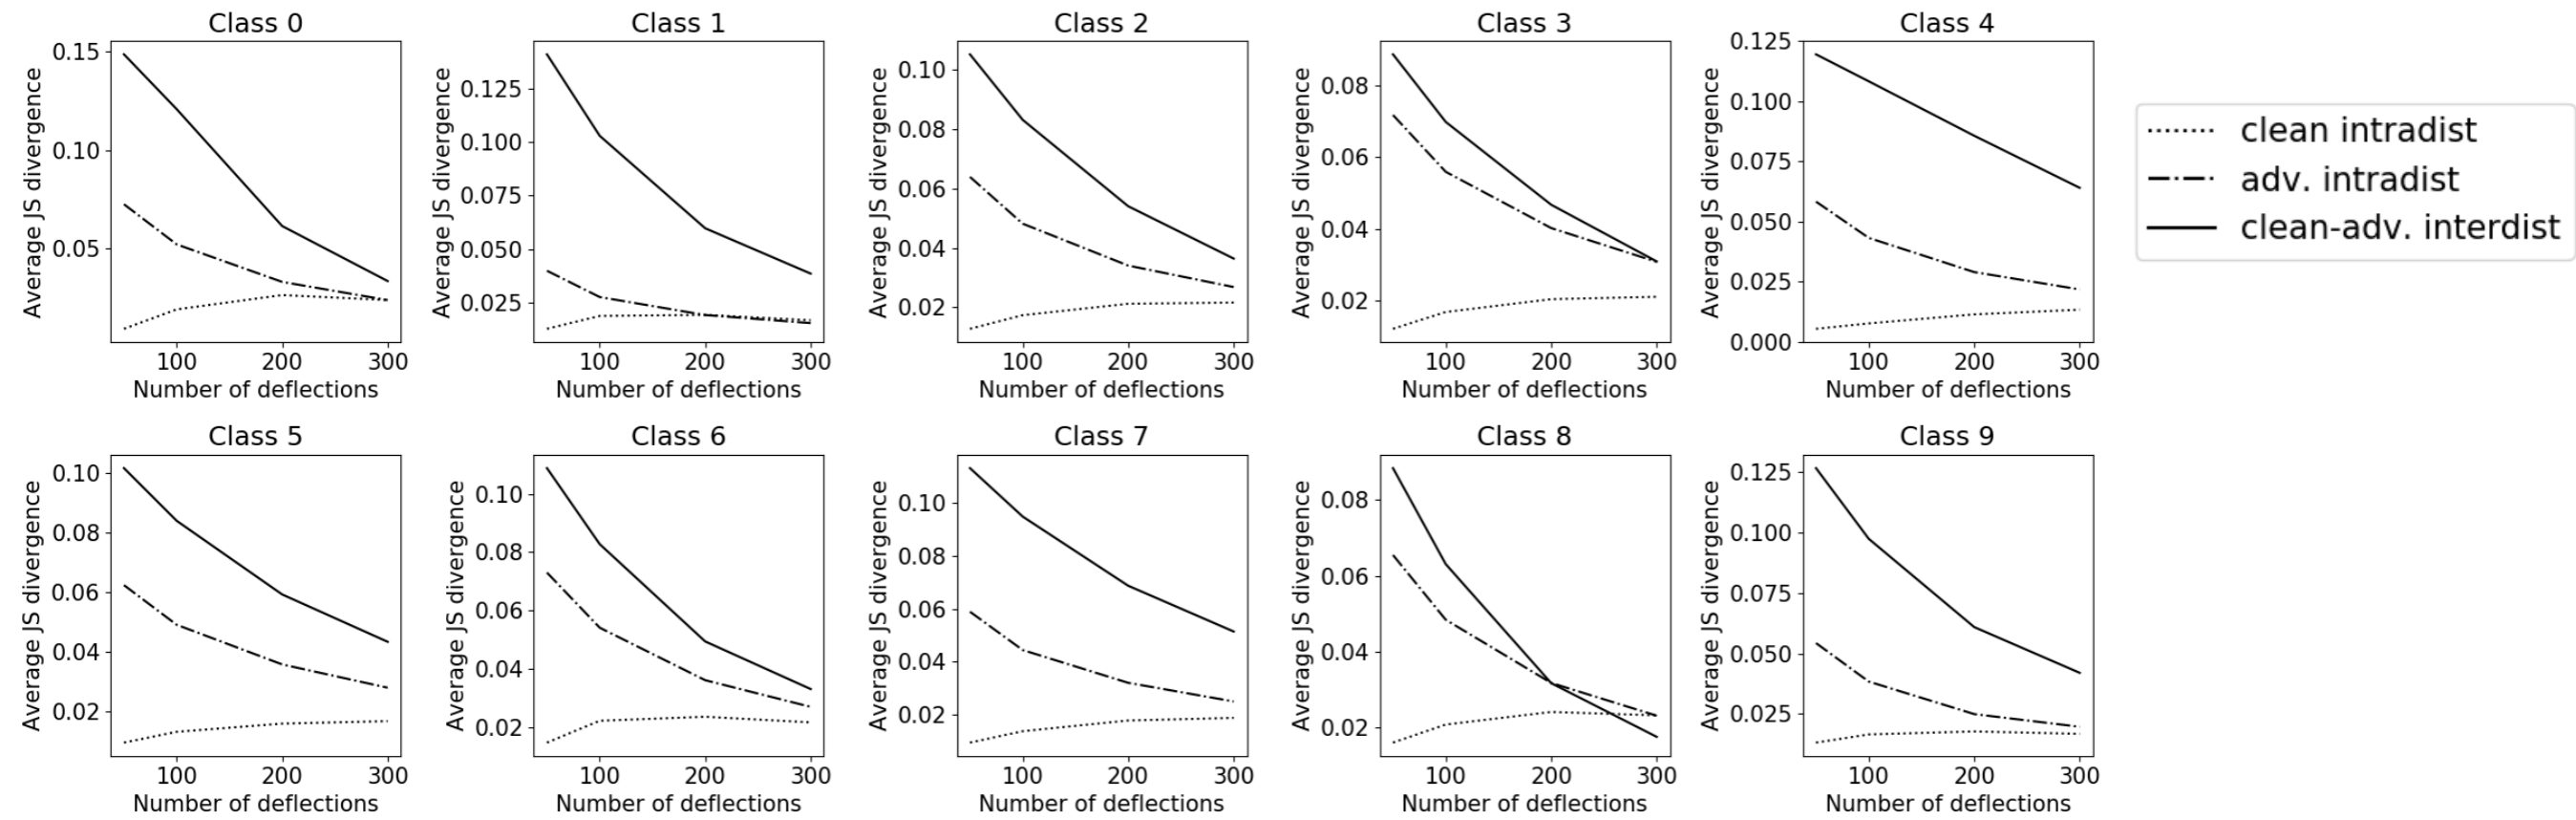

**clean**

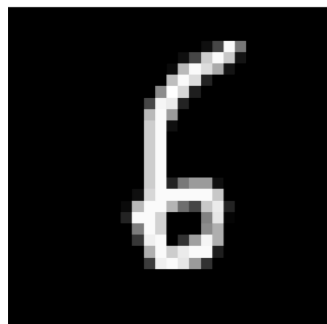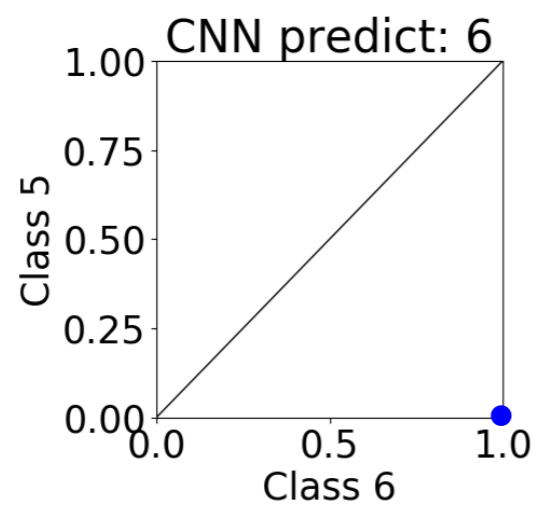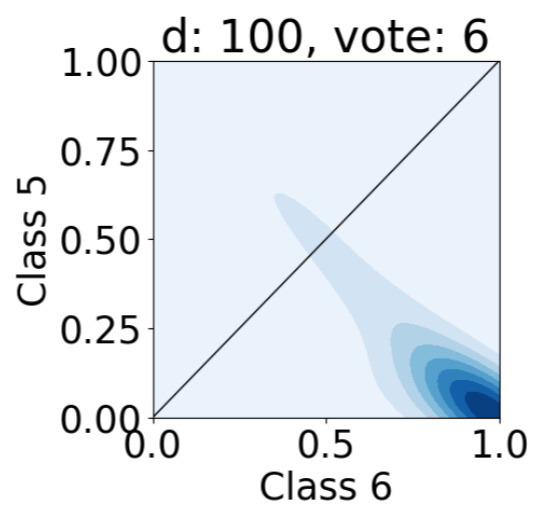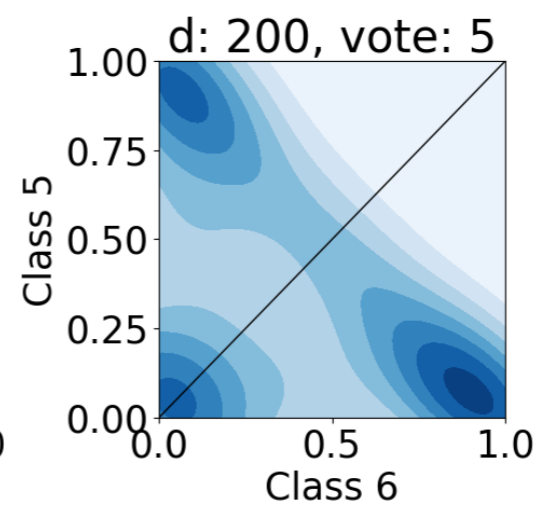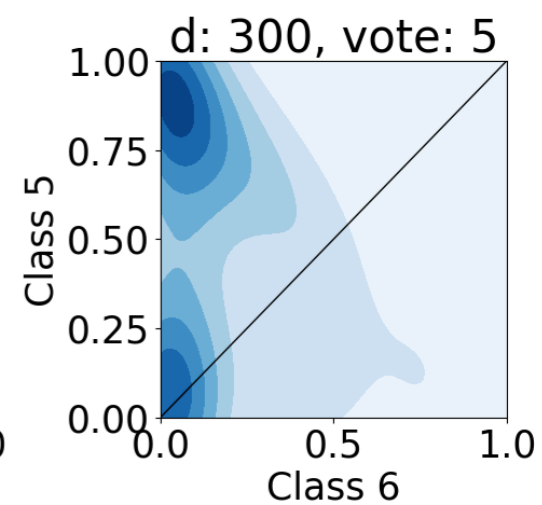

**adversarial**

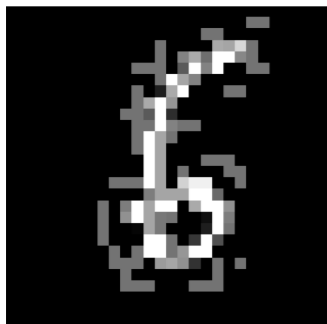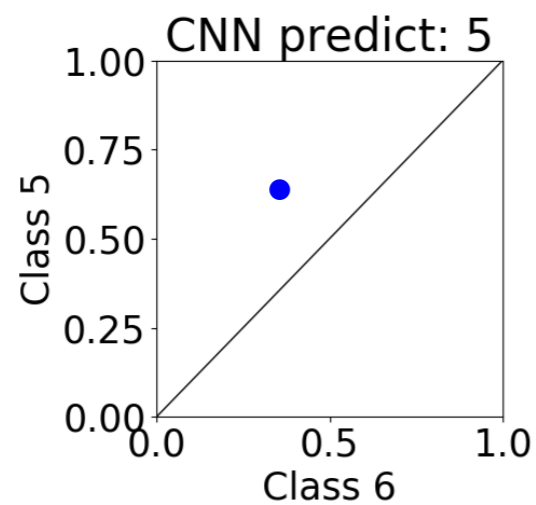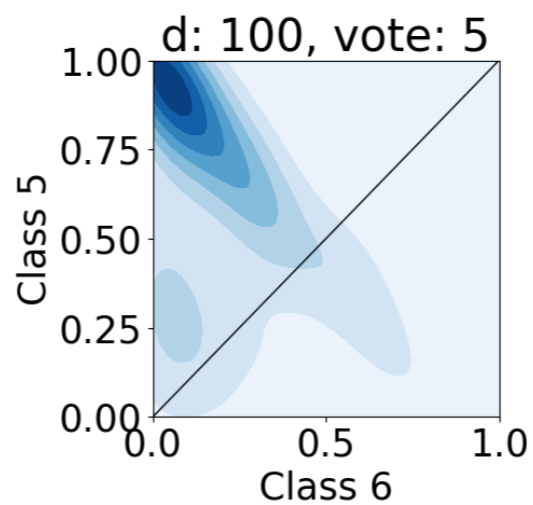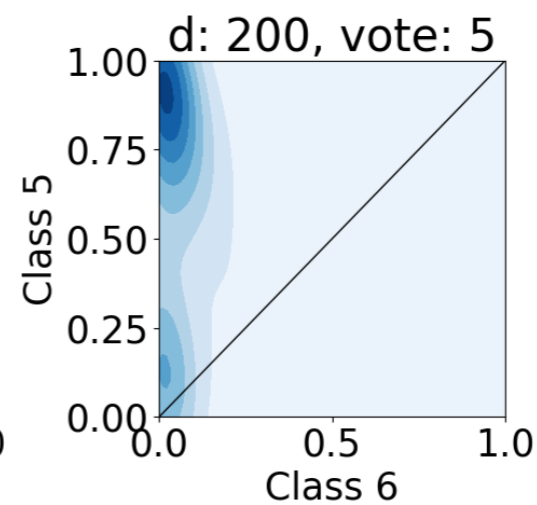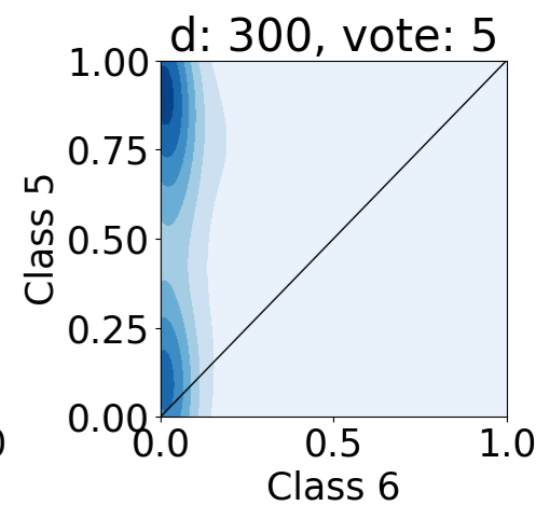

No perturbation

Increasing image transform

# MNIST FGSM PD RF

**clean**  
vote correct

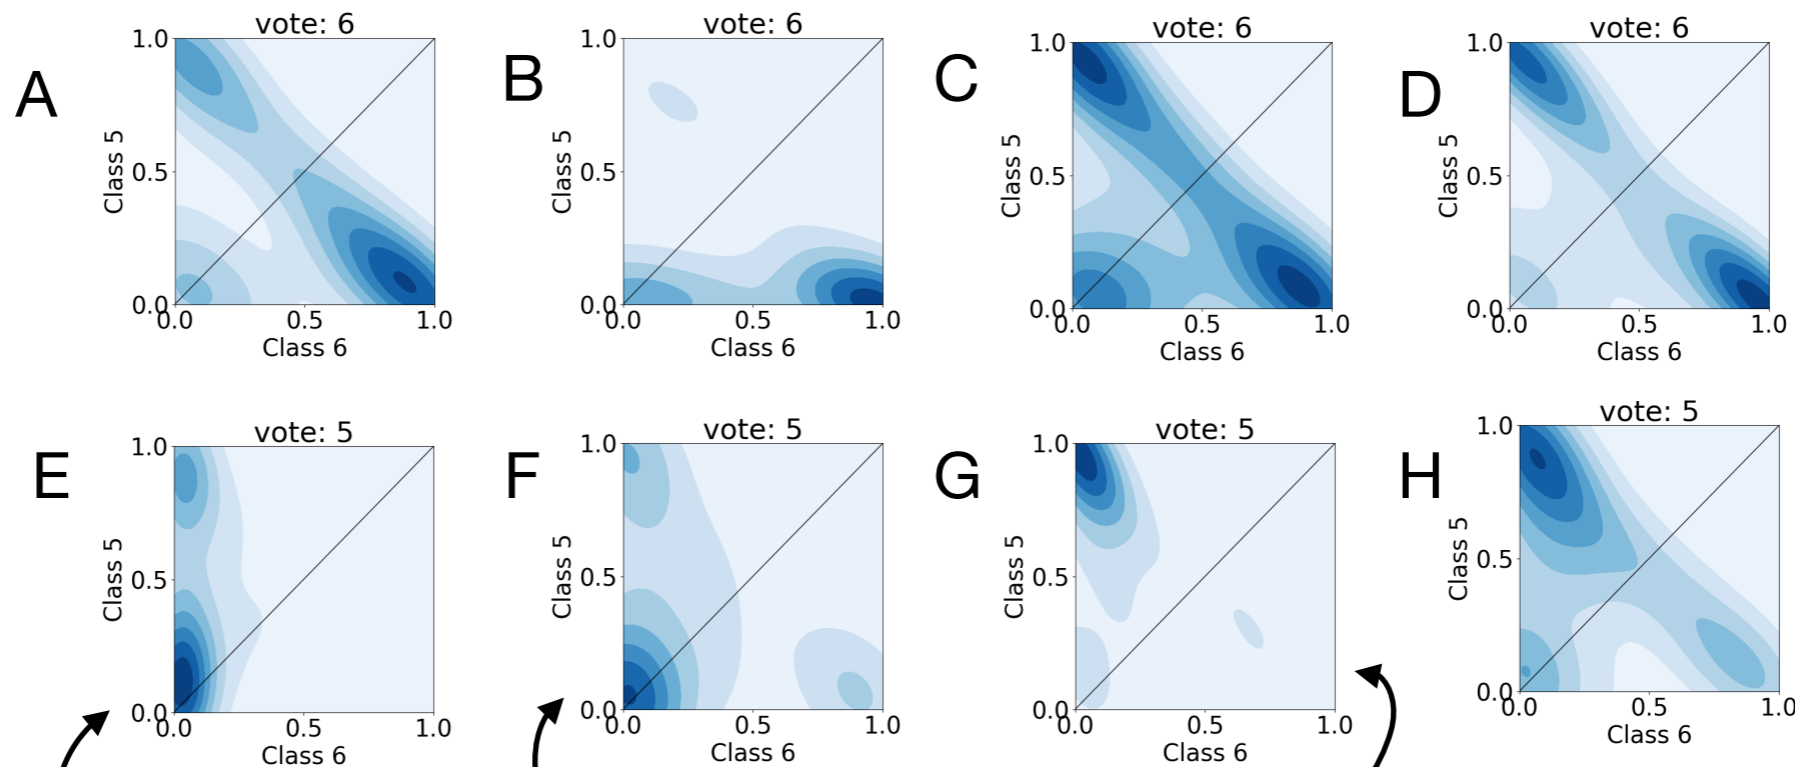

**adv.**  
vote wrong

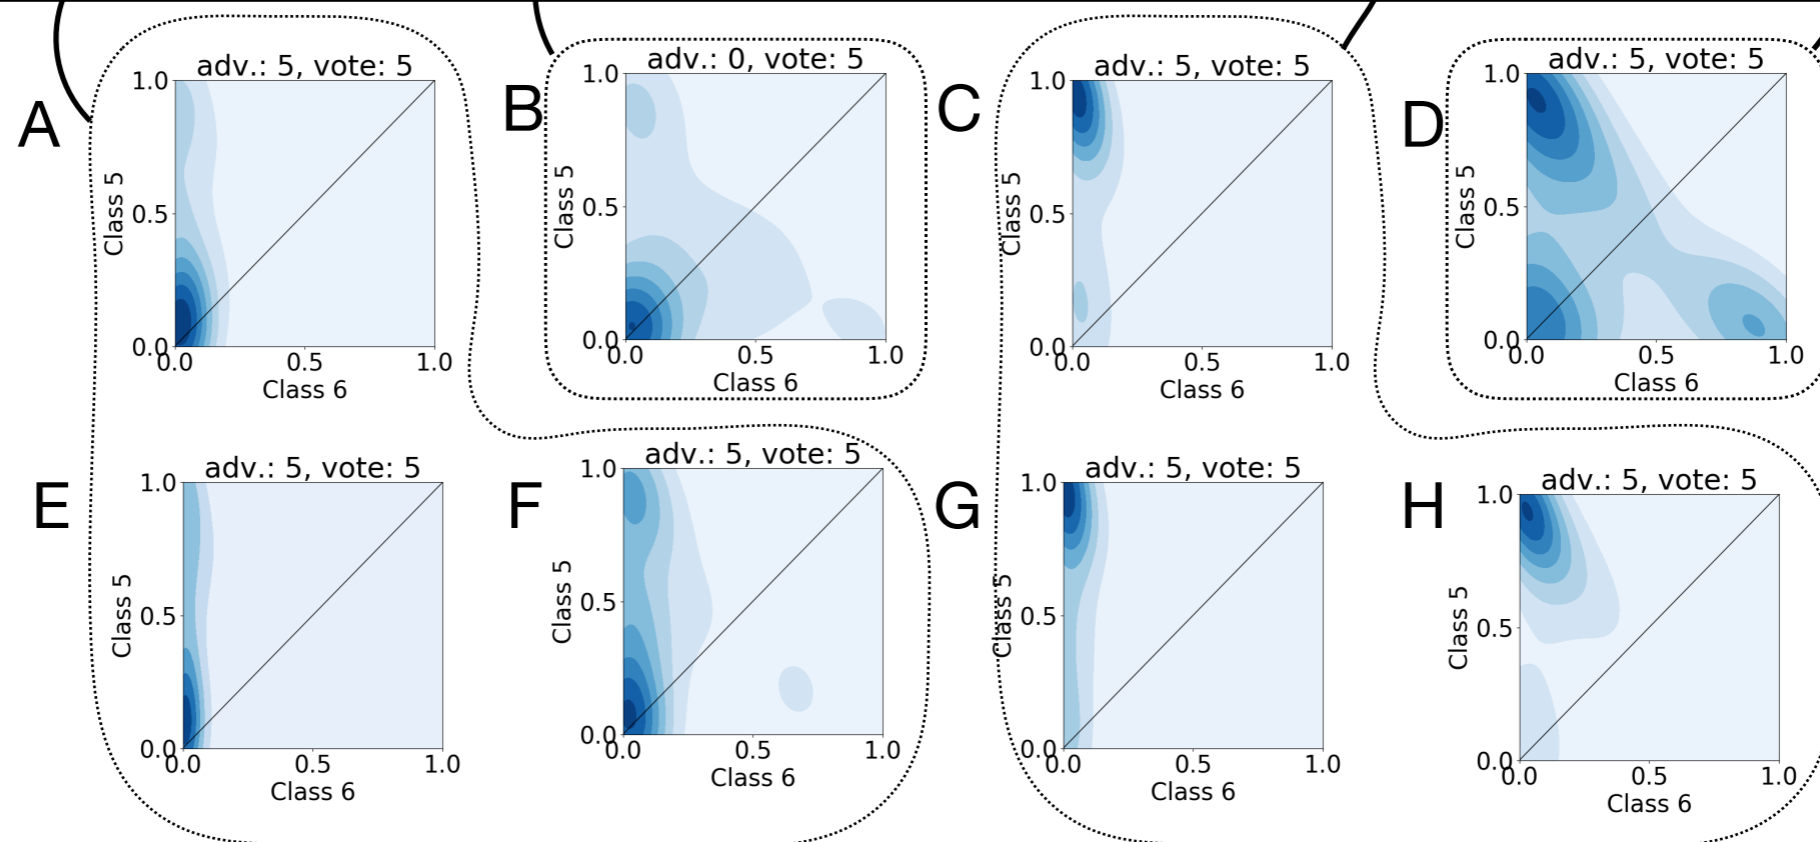

**Legit 5, DC correct**

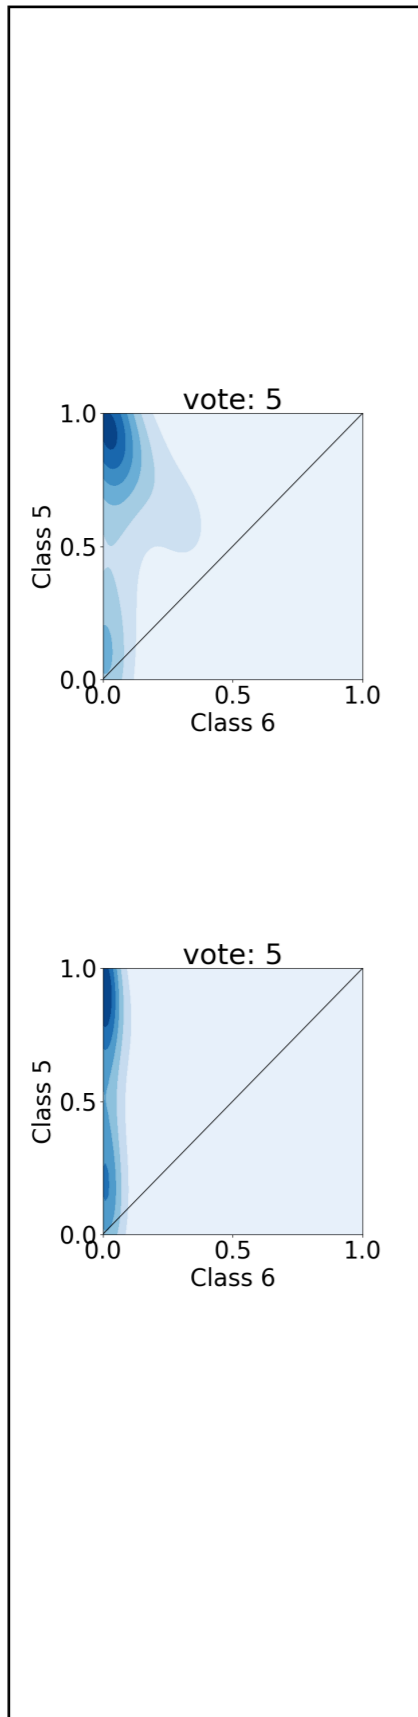

**label 6, adv, vote recovered, DC correct**

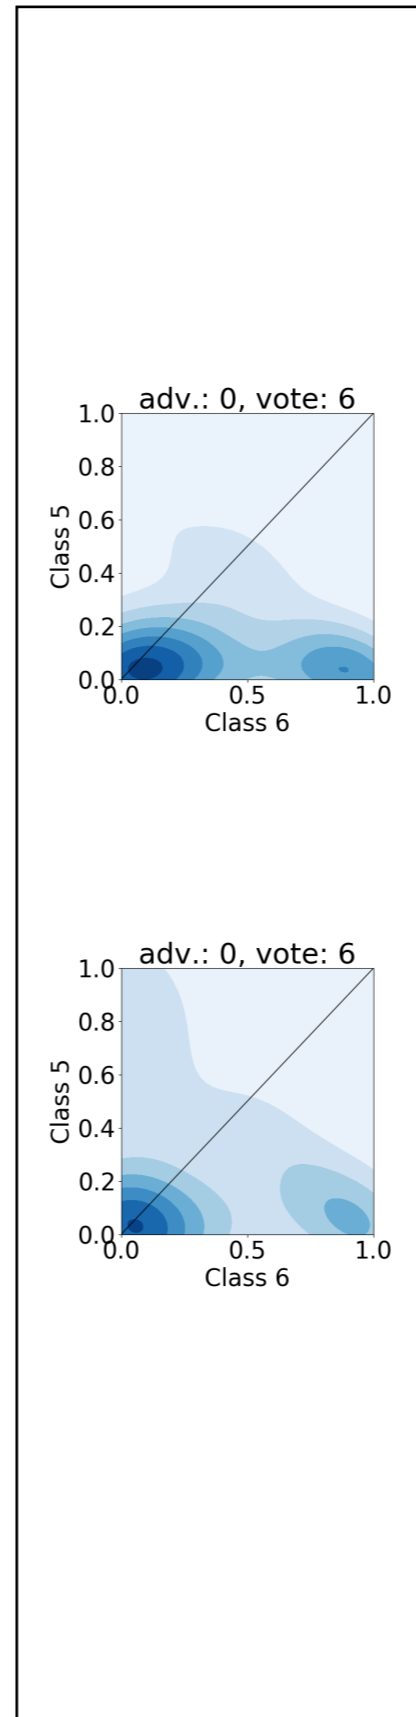

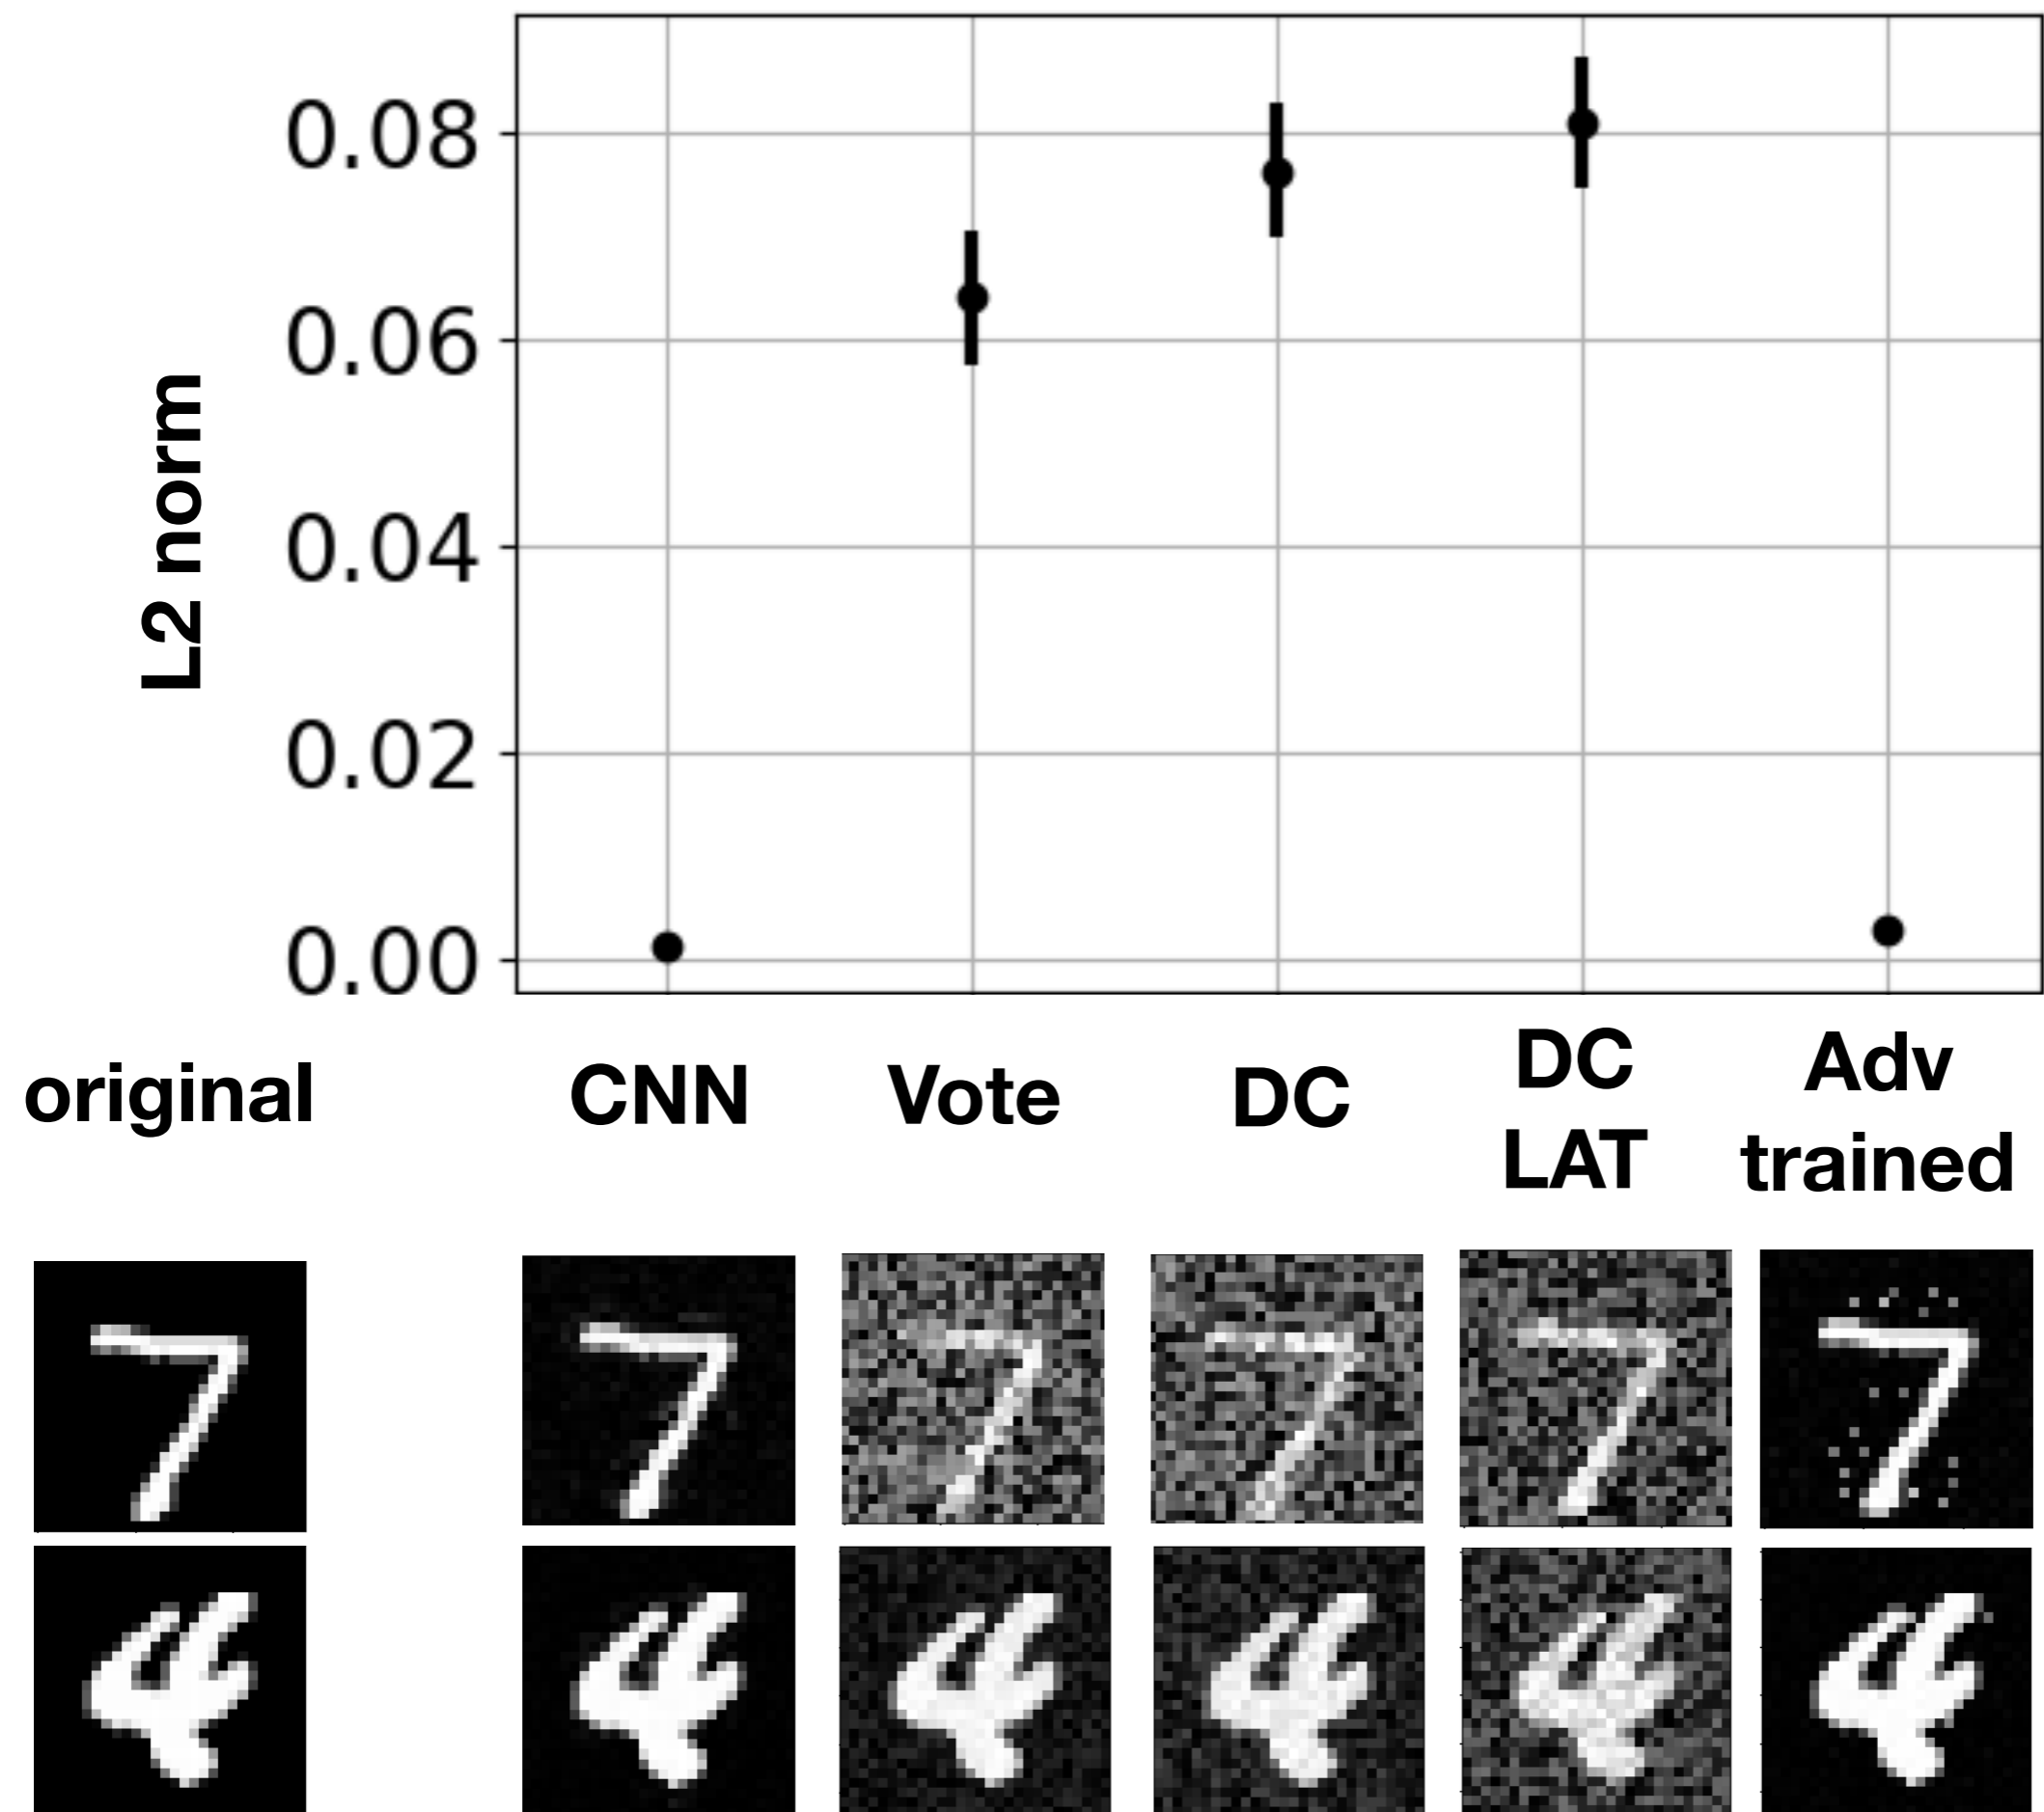

L2 norm

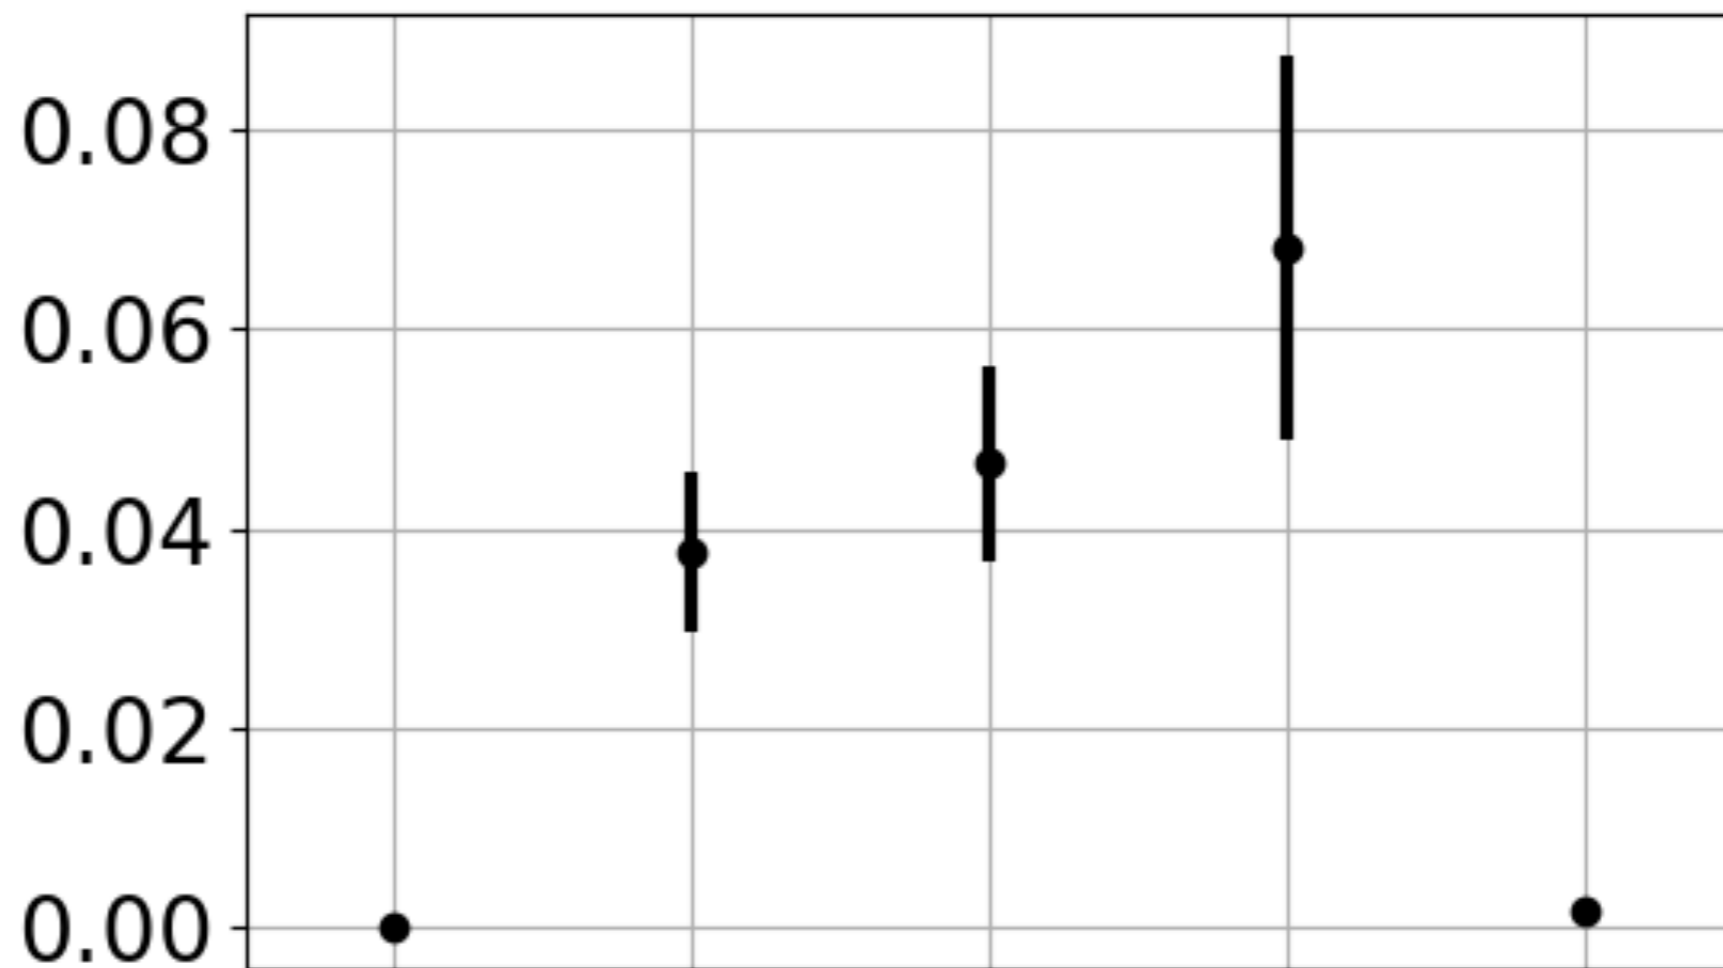

original

CNN

Vote

DC

DC  
LAT

Adv  
trained

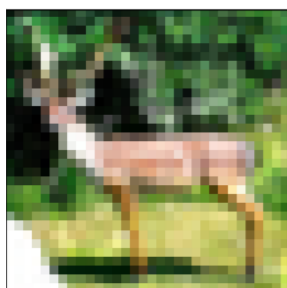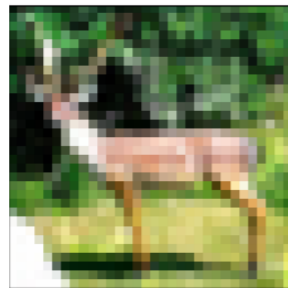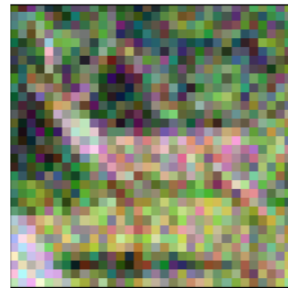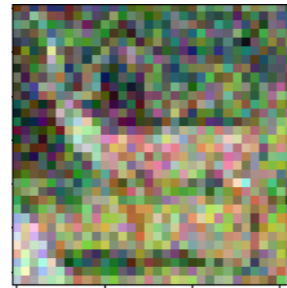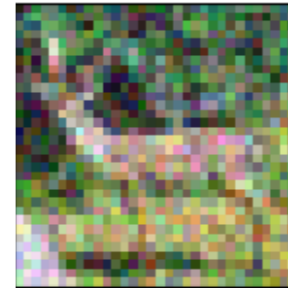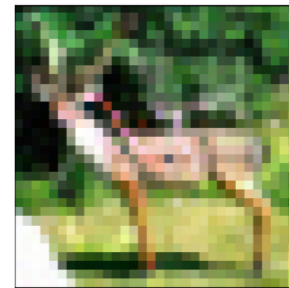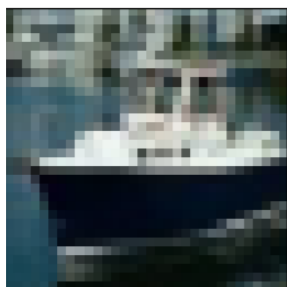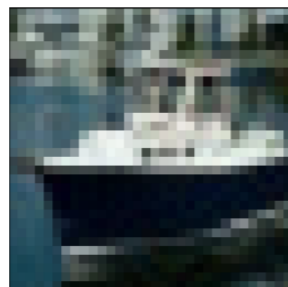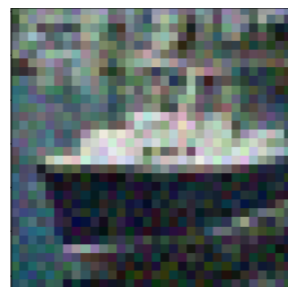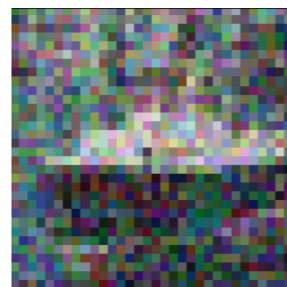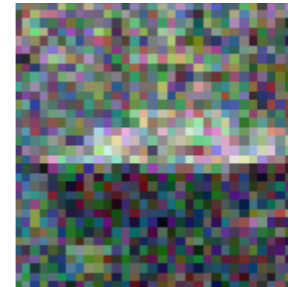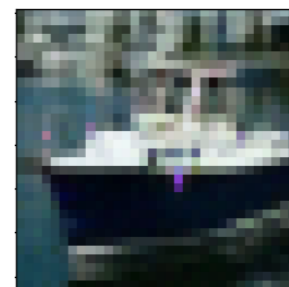

Supplement: Supplementary file 1 [file 20190916_additional_plots.pdf]
